# Supplementary material for: Bicircular Light Induced Multi-State Geometric Current
Source: arXiv:2503.03393 source file (2025-03-05)
Supplement: Supplementary file 1 [file appendix5_old.tex]

\section{Identification of Geometry Quantities for Shift Current} \label{Identification of Geometry Quantities for Shift Current_old_version}
		Similar to injection current, the shift current can also be categorized according to their inner geometry quantities. We separate this diagrams into seven parts: (shift vector dipole)$\times$(quantum geometric tensor), (shift vector)$\times$(shift vector)$\times$(quantum geometric tensor), (shift vector)$\times$(group velocity)$\times$(quantum geometric tensor), (group velocity)$\times$(group velocity)$\times$(quantum geometric tensor), (effective mass)$\times$(quantum geometric tensor), (group velocity)$\times$(triple phase product), (shift vector)$\times$(triple phase product). It's also worth noting that we only retain the resonant part here. 
        \par
        Here we encounter two types of generalized derivative, i.e. $h^{\gamma}_{ab; \mu}$, and $h^{\beta\gamma}_{ab; \mu}$. Diagram Set I contains both types and only the first type exist in Diagram Set II. To identify geometry quantities for these terms, it's convenient to introduce a separation strategy. In general, we expand covariant derivative term by their inner gauge covariant terms and gauge invariant terms. After taking derivative to both kinds, it's always possible to combine derivative over gauge covariant term with $(r^{\mu}_{aa} - r^{\mu}_{bb})$ to construct shift vector jointly.
        \par
        Let's take the easier generalized derivative $\partial_{\mu}h^{\gamma}_{ab} - i \left(r^{\mu}_{aa} - r^{\mu}_{bb}\right)h^{\gamma}_{ab}$ as an example. When band indices satisfies $a\neq b$, the first order covariant derivative can be written as $h^{\gamma}_{ab} = i\varepsilon_{ab}r^{\gamma}_{ab}$. The gauge invariant term here is $\varepsilon_{ab}$ and the gauge covariant term is $r^{\gamma}_{ab}$. Using the above strategy, we can reduce this term as
        \begin{equation}
            \label{expansion of first order generalized derivative}
            h^{\gamma}_{ab; \mu} = \left\{\Delta^{\mu}_{ab}\frac{h^{\gamma}_{ab}}{\varepsilon_{ab}}\right\} + \left\{-iR^{\mu, \gamma}_{ab}h^{\gamma}_{ab}\right\}
        \end{equation}
		\par
		The let's turn to the more complicated term $\partial_{\mu}h^{\beta\gamma}_{ab} - i(r^{\mu}_{aa} - r^{\mu}_{bb})h^{\beta\gamma}_{ab}$. Following the spirit of above strategy, $h^{\beta\gamma}_{ab}$ can be expressed as
		\begin{equation}
			\begin{aligned}
				h^{\beta\gamma}_{ab} = \varepsilon_{ab}R^{\beta, \gamma}_{ab} r^{\gamma}_{ab} + i\Delta^{\beta}_{ab}r^{\gamma}_{ab} + i\Delta^{\gamma}_{ab}r^{\beta}_{ab} + \sum\limits_{c, a\neq c \neq b}\left(\varepsilon_{cb}r^{\beta}_{ac} r^{\gamma}_{cb} - \varepsilon_{ac}r^{\gamma}_{ac}r^{\beta}_{cb}\right)
			\end{aligned}
		\end{equation}
		We find this expression consists of both gauge invariant terms and gauge covariant terms. The derivative can act on gauge invariant terms, i.e. $\varepsilon_{ab}$, $R^{\beta, \gamma}_{ab}$, $\Delta^{\beta}_{ab}$, or gauge covariant terms, i.e. $r^{\gamma}_{ab}$. When the derivative acts on gauge covariant terms, they can form a shift vector with $(r^{\mu}_{aa} - r^{\mu}_{bb})$.
        \par
        Then we can divide another generalized derivative $h^{\beta\gamma}_{ab; \mu}$ as
        \begin{equation}
            \label{expansion of second order generalized derivative}
            \begin{aligned}
                h^{\beta\gamma}_{ab; \mu}
                =& \left\{-ih^{\gamma}_{ab}\partial_{\mu}R^{\beta, \gamma}_{ab}\right\}  + \left\{-i\frac{\Delta^{\mu}_{ab}}{\varepsilon_{ab}}R^{\beta, \gamma}_{ab} h^{\gamma}_{ab} - i\Delta^{\beta}_{ab}R^{\mu, \gamma}_{ab}\frac{h^{\gamma}_{ab}}{\varepsilon_{ab}} - i\Delta^{\gamma}_{ab}R^{\mu, \beta}_{ab}\frac{h^{\beta}_{ab}}{\varepsilon_{ab}} \right\} \\
                &+ \left\{-R^{\beta, \gamma}_{ab} R^{\mu,\gamma}_{ab}h^{\gamma}_{ab}\right\} + \left\{ w^{\mu\beta}_{ab}\frac{h^{\gamma}_{ab}}{\varepsilon_{ab}}  +  w^{\mu\gamma}_{ab}\frac{h^{\beta}_{ab}}{\varepsilon_{ab}}\right\} \\
                &+ \sum\limits_{c, a\neq c \neq b} \left[\left\{-\Delta^{\mu}_{cb}\frac{h^{\beta}_{ac} h^{\gamma}_{cb}}{\varepsilon_{ac}\varepsilon_{cb}} + \Delta^{\mu}_{ac}\frac{h^{\gamma}_{ac} h^{\beta}_{cb}}{\varepsilon_{ac}\varepsilon_{cb}}\right\}  + \left\{i\left(R^{\mu, \beta}_{ac}+ R^{\mu, \gamma}_{cb}\right) \frac{h^{\beta}_{ac}h^{\gamma}_{cb}}{\varepsilon_{ac}} + i\left(R^{\mu, \gamma}_{ac}+ R^{\mu, \beta}_{cb}\right)\frac{h^{\gamma}_{ac}h^{\beta}_{cb}}{\varepsilon_{cb}}\right\}\right]
            \end{aligned}
        \end{equation}
        After using this strategy, the underlying quantum geometry becomes clear. Details of categorization are list below.
        
		\paragraph{Part 1: (quantum geometric tensor)$\times$(shift vector dipole)}
		This term can be obtained by conducting derivative on gauge invariant term $R^{\beta, \gamma}_{ab}$, the first term in Equation \ref{expansion of second order generalized derivative}.
		\begin{equation}
			\begin{aligned}
				\sigma^{\mu\alpha\beta\gamma}_{\text{BCL, $\partial$R$\times$Q}} =& 	\frac{1}{3!}\frac{ie^4}{2\hbar^4\omega_1\omega_2\omega_3}\sum\limits_{\{\alpha, \beta, \gamma\}}\sum\limits_{\{(\alpha, \omega_1), (\beta, \omega_2), (\gamma, \omega_3)\}} \sum\limits_{ab} \int [d\boldsymbol{k}]f_{ab}h^{\alpha}_{ba}\left(-ih^{\gamma}_{ab}\partial_{\mu}R^{\beta,\gamma}_{ab}\right)d^{\omega_1}_{ab} \\
				=& \frac{1}{3!}\frac{i\pi e^4}{2\hbar^4\Omega^3}\sum\limits_{\{\alpha, \beta, \gamma\}} \sum\limits_{ab} \int [d\boldsymbol{k}]f_{ab}h^{\alpha}_{ba}h^{\gamma}_{ab} \left[2\partial_{\mu}R^{\beta,\gamma}_{ab} \delta(\varepsilon_{ab} + \Omega) -  \partial_{\mu}R^{\beta,\alpha}_{ba} \delta(\varepsilon_{ab} + 2\Omega)\right]
			\end{aligned}
		\end{equation}

        \paragraph{Part 2: (shift vector)$\times$(shift vector)$\times$(quantum geometric tensor)}There are two origin of such term, both in Diagram Set I, (i) extracting the third term in Equation \ref{expansion of second order generalized derivative}
		\begin{equation}
			\begin{aligned}
				\sigma^{\mu\alpha\beta\gamma}_{\text{BCL, $\text{R}^2\times$Q}-1}
				=& \frac{1}{3!}\frac{ie^4}{2\hbar^4\omega_1\omega_2\omega_3}\sum\limits_{\{\alpha, \beta, \gamma\}}\sum\limits_{\{(\alpha, \omega_1), (\beta, \omega_2), (\gamma, \omega_3)\}} \sum\limits_{ab} \int [d\boldsymbol{k}]\left[f_{ab}h^{\alpha}_{ba}h^{\gamma}_{ab}\left(-R^{\beta,\gamma}_{ab}R^{\mu,\gamma}_{ab}\right)d^{\omega_1}_{ab} \right]
			\end{aligned}
		\end{equation}		
        (ii) extracting the second term in Equation \ref{expansion of first order generalized derivative} and $h^{\beta}_{ba}$ from $h^{\alpha\beta}_{ba}$.
		\begin{equation}
			\begin{aligned}
				\sigma^{\mu\alpha\beta\gamma}_{\text{BCL, $\text{R}^2\times$Q}-2} =& \frac{1}{3!}\frac{i e^4}{2\hbar^4\omega_1\omega_2\omega_3}\sum\limits_{\{\alpha, \beta, \gamma\}}\sum\limits_{\{(\alpha, \omega_1), (\beta, \omega_2), (\gamma, \omega_3)\}} \sum\limits_{ab} \int [d\boldsymbol{k}]\left[f_{ab}\left(-ih^{\beta}_{ba}R^{\alpha,\beta}_{ba}\right)\left(-ih^{\gamma}_{ab}R^{\mu,\gamma}_{ab}\right)d^{\omega_{12}}_{ab}\right] \\
			\end{aligned}
		\end{equation}		
        Add up both terms, we can obtain the overall expression:
		\begin{equation}
			\begin{aligned}
				\sigma^{\mu\alpha\beta\gamma}_{\text{BCL, $\text{R}^2\times$Q}} =& -\frac{1}{3!}\frac{ie^4}{2\hbar^4\omega_1\omega_2\omega_3}\sum\limits_{\{\alpha, \beta, \gamma\}}\sum\limits_{\{(\alpha, \omega_1), (\beta, \omega_2), (\gamma, \omega_3)\}} \sum\limits_{ab} \int [d\boldsymbol{k}]\left[f_{ab}h^{\alpha}_{ba}h^{\gamma}_{ab}\left(R^{\beta,\gamma}_{ab}R^{\mu,\gamma}_{ab} -R^{\beta,\gamma}_{ab} R^{\mu,\alpha}_{ba}\right)d^{\omega_{1}}_{ab}\right] \\
				=& -\frac{1}{3!}\frac{ie^4}{2\hbar^4\omega_1\omega_2\omega_3}\sum\limits_{\{\alpha, \beta, \gamma\}}\sum\limits_{\{(\alpha, \omega_1), (\beta, \omega_2), (\gamma, \omega_3)\}} \sum\limits_{ab} \int [d\boldsymbol{k}]\left[f_{ab}h^{\alpha}_{ba}h^{\gamma}_{ab}R^{\beta,\gamma}_{ab}\left(R^{\mu,\gamma}_{ab} - R^{\mu,\alpha}_{ba}\right)d^{\omega_{1}}_{ab}\right] \\
				=& \frac{1}{3!}\frac{\pi e^4}{2\hbar^4\Omega^3}\sum\limits_{\{\alpha, \beta, \gamma\}} \sum\limits_{ab} \int [d\boldsymbol{k}]f_{ab}h^{\alpha}_{ba}h^{\gamma}_{ab} \left(R^{\mu,\gamma}_{ab} - R^{\mu,\alpha}_{ba}\right)
				\left[ 2R^{\beta,\gamma}_{ab}\delta(\varepsilon_{ab} + \Omega) + R^{\beta,\alpha}_{ba}\delta(\varepsilon_{ab} + 2\Omega) \right]				
			\end{aligned}
		\end{equation}

		\paragraph{Part 3: (group velocity)$\times$(shift vector)$\times$(quantum geometric tensor)} We will show that both Diagram Set I and Diagram Set II contribute to such term. For Diagram Set I, we can derive such term by two ways, i.e. (i) extract the second term in Equation \ref{expansion of second order generalized derivative}
		\begin{equation}
			\begin{aligned}
				\sigma^{\mu\alpha\beta\gamma}_{\text{BCL, } \Delta\times\text{R}\times\text{Q-1}} =& \frac{1}{3!}\frac{ie^4}{2\hbar^4\omega_1\omega_2\omega_3}\sum\limits_{\{\alpha, \beta, \gamma\}}\sum\limits_{\{(\alpha, \omega_1), (\beta, \omega_2), (\gamma, \omega_3)\}} \sum\limits_{ab} \int [d\boldsymbol{k}]f_{ab}h^{\alpha}_{ba}\Delta^{\mu}_{ab} \\
                &\left(-i\frac{\Delta^{\mu}_{ab}}{\varepsilon_{ab}}R^{\beta, \gamma}_{ab} h^{\gamma}_{ab} - i\Delta^{\beta}_{ab}R^{\mu, \gamma}_{ab}\frac{h^{\gamma}_{ab}}{\varepsilon_{ab}} - i\Delta^{\gamma}_{ab}R^{\mu, \beta}_{ab}\frac{h^{\beta}_{ab}}{\varepsilon_{ab}} \right)r^{\gamma}_{ab}d^{\omega_1}_{ab} \\
				=&\frac{1}{3!}\frac{i\pi e^4}{2\hbar^4\Omega^3}\sum\limits_{\{\alpha, \beta, \gamma\}}\sum\limits_{ab} \int [d\boldsymbol{k}]f_{ab}\frac{h^{\alpha}_{ba}h^{\gamma}_{ab}}{\varepsilon_{ab}}\left\{\Delta^{\mu}_{ab}\left[2R^{\beta, \gamma}_{ab}\delta(\varepsilon_{ab} + \Omega) - R^{\beta, \alpha}_{ba}\delta(\varepsilon_{ab} + 2\Omega)\right] \right.\\
                &\left.+2\Delta^{\beta}_{ab}\left[ 2R^{\mu, \gamma}_{ab}\delta(\varepsilon_{ab}+ \Omega) -R^{\mu, \alpha}_{ba}\delta(\varepsilon_{ab}+ 2\Omega) \right]\right\}
			\end{aligned}
		\end{equation}
		\par
		(ii) extract the first part of Equation \ref{expansion of first order generalized derivative} and combine it with $-iR^{\alpha, \beta}_{ba}h^{\beta}_{ba}$ in the $h^{\alpha\beta}_{ba}$, and extract the second part of of Equation \ref{expansion of first order generalized derivative} and combine it with $(\Delta^{\alpha}_{ba}h^{\beta}_{ba} + \Delta^{\beta}_{ba}h^{\alpha}_{ba})/ \varepsilon_{ba}$ in the $h^{\alpha\beta}_{ba}$. The result turns out to be
		\begin{equation}
			\begin{aligned}
				\sigma^{\mu\alpha\beta\gamma}_{\text{BCL, } \Delta\times\text{R}\times\text{Q} - 2} =& \frac{1}{3!}\frac{ie^4}{2\hbar^4\omega_1\omega_2\omega_3}\sum\limits_{\{\alpha, \beta, \gamma\}}\sum\limits_{\{(\alpha, \omega_1), (\beta, \omega_2), (\gamma, \omega_3)\}} \sum\limits_{ab} \int [d\boldsymbol{k}] \\
				&f_{ab}d^{\omega_{12}}_{ab} \left\{i\Delta^{\alpha}_{ba}h^{\beta}_{ba} R^{\mu, \gamma}_{ab}\frac{h^{\gamma}_{ab}}{\varepsilon_{ab}} - i\Delta^{\beta}_{ba}h^{\alpha}_{ba} R^{\mu, \gamma}_{ab}\frac{h^{\gamma}_{ab}}{ \varepsilon_{ab}} + iR^{\alpha, \beta}_{ba}h^{\beta}_{ba} i \Delta^{\mu}_{ab}\frac{h^{\gamma}_{ab}}{\varepsilon_{ab}}\right\} \\
				=& -\frac{1}{3!}\frac{i\pi e^4}{2\hbar^4\Omega^3}\sum\limits_{\{\alpha, \beta, \gamma\}}\sum\limits_{ab} \int [d\boldsymbol{k}]  2f_{ab}\frac{h^{\alpha}_{ba}h^{\gamma}_{ab}}{\varepsilon_{ab}}\left\{\Delta^{\beta}_{ab}\left[2R^{\mu, \alpha}_{ba}\delta(\varepsilon_{ab}+ \Omega) -R^{\mu, \gamma}_{ab}\delta(\varepsilon_{ab}+ 2\Omega) \right]\right.\\
				&+ \left.\Delta^{\mu}_{ab}\left[2R^{\beta, \alpha}_{ba}\delta(\varepsilon_{ab}+ \Omega) -R^{\beta, \gamma}_{ab}\delta(\varepsilon_{ab}+ 2\Omega) \right]\right\}\\
			\end{aligned}
		\end{equation}
		\par
		Add up both terms, we can obtain the contribution from Diagram Set I
		\begin{equation}
			\begin{aligned}
				\sigma^{\mu\alpha\beta\gamma}_{\text{BCL, } \Delta\times\text{R}\times\text{Q, I}} =& \frac{1}{3!}\frac{i\pi e^4}{2\hbar^4\Omega^3}\sum\limits_{\{\alpha, \beta, \gamma\}}\sum\limits_{ab} \int [d\boldsymbol{k}] f_{ab}\frac{h^{\alpha}_{ba}h^{\gamma}_{ab}}{\varepsilon_{ab}}\\ &\left[2\Delta^{\beta}_{ab}\left(R^{\mu, \gamma}_{ab} - R^{\mu, \alpha}_{ba}\right) + \Delta^{\mu}_{ab}\left(R^{\beta, \gamma}_{ab} - R^{\beta, \alpha}_{ba}\right)\right]\left(2\delta(\varepsilon_{ab}+ \Omega) +\delta(\varepsilon_{ab}+ 2\Omega)\right)\\
			\end{aligned}
		\end{equation}	
        \par
        For Diagram II, we can obtain such term by requiring band indices $(a\neq c, a=b)$ and $(a\neq c, b=c)$. Start from Equation \ref{Shift current Diagram Set II} and exert above requirement, we can obtain
		\begin{equation}
			\begin{aligned}
				\sigma^{\mu\alpha\beta\gamma}_{\text{BCL, II,  b=a}}
				=&\frac{1}{3!}\frac{ie^4}{\hbar^4\omega_1\omega_2\omega_3}\sum\limits_{\{\alpha, \beta, \gamma\}}\sum\limits_{\{(\alpha, \omega_1), (\beta, \omega_2), (\gamma, \omega_3)\}} \sum\limits_{a \neq c} \int [d\boldsymbol{k}] \\
				&\left[\left(-iR^{\mu, \gamma}_{ac}+ \frac{\Delta^{ac}_{ac}}{\varepsilon_{ac}}\right)h^{\alpha}_{aa}h^{\beta}_{ca}h^{\gamma}_{ac}\right]\times(-i\pi)\left[ f_{ac} d^{\omega_{1}}_{aa} \delta(\varepsilon_{ac} + \omega_{12}) - f_{ac} d^{\omega_{1}}_{aa} \delta(\varepsilon_{ac} + \omega_2)\right] \\
			\end{aligned}
		\end{equation}
		\begin{equation}
			\begin{aligned}
				\sigma^{\mu\alpha\beta\gamma}_{\text{BCL, II,  b=c}}
				=&\frac{1}{3!}\frac{ie^4}{\hbar^4\omega_1\omega_2\omega_3}\sum\limits_{\{\alpha, \beta, \gamma\}}\sum\limits_{\{(\alpha, \omega_1), (\beta, \omega_2), (\gamma, \omega_3)\}} \sum\limits_{a \neq c} \int [d\boldsymbol{k}] \\
				&\left[\left(-iR^{\mu, \gamma}_{ac}+\frac{\Delta^{\mu}_{ac}}{\varepsilon_{ac}}\right)h^{\alpha}_{ca}h^{\beta}_{cc}h^{\gamma}_{ac}\right]\times(-i\pi)\left[f_{ac} d^{\omega_{2}}_{aa} \delta(\varepsilon_{ac} + \omega_1) - f_{ac} d^{\omega_{2}}_{aa} \delta(\varepsilon_{ac} + \omega_{12})\right] \\
			\end{aligned}
		\end{equation}
		Sum up both terms, we can obtain the overall contribution from the Diagram Set II 
		\begin{equation}
			\begin{aligned}
				\sigma^{\mu\alpha\beta\gamma}_{\text{BCL, R$\times\Delta\times$Q, II}}
				=&\frac{1}{3!}\frac{\pi ie^4}{2\hbar^4\Omega^3}\sum\limits_{\{\alpha, \beta, \gamma\}}\sum\limits_{ab} \int [d\boldsymbol{k}] \\
				&\left[f_{ab}\left(R^{\mu, \gamma}_{ab} - R^{\mu, \beta}_{ba}\right)\frac{h^{\beta}_{ba}h^{\gamma}_{ab}}{\varepsilon_{ab}}\Delta^{\alpha}_{ab}\right]\left[\delta(\varepsilon_{ab} + \Omega) - 4 \delta(\varepsilon_{ab} + 2\Omega)\right] \\
			\end{aligned}
		\end{equation}
        Here we apply the similar approximation used in Appendix \ref{Identification of Geometry Quantities for Injection Current} that we can safely neglect the relaxation time term in the denominator of $d^{\omega}_{aa}$.
        \par
        Now, we have found all the related terms and the overall expression is
        \begin{equation}
			\begin{aligned}
				\sigma^{\mu\alpha\beta\gamma}_{\text{BCL, R$\times\Delta\times$Q}}
				=&\frac{1}{3!}\frac{i\pi e^4}{2\hbar^4\Omega^3}\sum\limits_{\{\alpha, \beta, \gamma\}}\sum\limits_{ab} \int [d\boldsymbol{k}] f_{ab}\frac{h^{\alpha}_{ba}h^{\gamma}_{ab}}{\varepsilon_{ab}}\left\{\left[2\Delta^{\beta}_{ab}\left(R^{\mu, \gamma}_{ab} - R^{\mu, \alpha}_{ba}\right)\right]\left(5\delta(\varepsilon_{ab}+ \Omega) -2\delta(\varepsilon_{ab}+ 2\Omega)\right)\right. \\
                &\left.+\left[\Delta^{\mu}_{ab}\left(R^{\beta, \gamma}_{ab} - R^{\beta, \alpha}_{ba}\right)\right]\left(2\delta(\varepsilon_{ab}+ \Omega) +\delta(\varepsilon_{ab}+ 2\Omega)\right)\right\}\\
			\end{aligned}
		\end{equation}
        
		\paragraph{Part 4: (group velocity)$\times$(group velocity)$\times$(quantum geometric tensor)} This term solely comes from Diagram Set I. The only way is extracting the first part of Equation \ref{expansion of first order generalized derivative}, then combining it with  $(\Delta^{\alpha}_{ba}h^{\beta}_{ba} + \Delta^{\beta}_{ba}h^{\alpha}_{ba})/ \varepsilon_{ba}$ in the $h^{\alpha\beta}_{ba}$.
		\begin{equation}
			\begin{aligned}
				\sigma^{\mu\alpha\beta\gamma}_{\text{BCL, } \Delta^2\times\text{Q}} =& \frac{1}{3!}\frac{ie^4}{2\hbar^4\omega_1\omega_2\omega_3}\sum\limits_{\{\alpha, \beta, \gamma\}}\sum\limits_{\{(\alpha, \omega_1), (\beta, \omega_2), (\gamma, \omega_3)\}} \sum\limits_{ab} \int [d\boldsymbol{k}]f_{ab} \left(\Delta^{\alpha}_{ba}\frac{h^{\beta}_{ba}}{\varepsilon_{ba}} + \Delta^{\beta}_{ba}\frac{h^{\alpha}_{ba}}{\varepsilon_{ba}}\right)\Delta^{\mu}_{ab}\frac{h^{\gamma}_{ab}}{\varepsilon_{ab}} d^{\omega_{12}}_{ab} \\
				=& \frac{1}{3!}\frac{\pi e^4}{\hbar^4 \Omega^3}\sum\limits_{\{\alpha, \beta, \gamma\}} \sum\limits_{ab} \int [d\boldsymbol{k}]f_{ab}\Delta^{\alpha}_{ab}\Delta^{\mu}_{ab}\frac{h^{\beta}_{ba}h^{\gamma}_{ab}}{\varepsilon^2_{ab}}\left[ 2\delta(\varepsilon_{ab} + \Omega) - \delta(\varepsilon_{ab} + 2\Omega)\right]
			\end{aligned}
		\end{equation}


		\paragraph{Part 5: (effective mass)$\times$(quantum geometric tensor)} This term can be obtained from both Diagram Set I and Diagram Set II. For Diagram Set I, this term corresponds to the forth part of Equation \ref{expansion of second order generalized derivative}.
		\begin{equation}
			\begin{aligned}
				\sigma^{\mu\alpha\beta\gamma}_{\text{BCL, $\text{m}\times$Q, I}} =& \frac{1}{3!}\frac{ie^4}{2\hbar^4\omega_1\omega_2\omega_3}\sum\limits_{\{\alpha, \beta, \gamma\}}\sum\limits_{\{(\alpha, \omega_1), (\beta, \omega_2), (\gamma, \omega_3)\}} \sum\limits_{ab} \int [d\boldsymbol{k}]f_{ab}h^{\alpha}_{ba}d^{\omega_1}_{ab}\left[w^{\mu\beta}_{ab}\frac{h^{\gamma}_{ab}}{\varepsilon_{ab}} + w^{\mu\gamma}_{ab}\frac{h^{\beta}_{ab}}{\varepsilon_{ab}}\right] \\
				=& -\frac{1}{3!}\frac{\pi e^4}{\hbar^4\Omega^3}\sum\limits_{\{\alpha, \beta, \gamma\}} \sum\limits_{ab} \int [d\boldsymbol{k}]f_{ab}\frac{h^{\alpha}_{ba}h^{\gamma}_{ab}}{\varepsilon_{ab}}w^{\mu\beta}_{ab}\left[2\delta(\varepsilon_{ab} + \Omega) - \delta(\varepsilon_{ab} + 2\Omega)\right]\\
			\end{aligned}
		\end{equation} 
        \par
		For Diagram Set II, this term is related to the case that $a=c$. In the case $a=c$, the corresponding expression is
		\begin{equation}
			\begin{aligned}
				\sigma^{\mu\alpha\beta\gamma}_{\text{BCL, II, a=c}}
				=&\frac{1}{3!}\frac{ie^4}{\hbar^4\omega_1\omega_2\omega_3}\sum\limits_{\{\alpha, \beta, \gamma\}}\sum\limits_{\{(\alpha, \omega_1), (\beta, \omega_2), (\gamma, \omega_3)\}} \sum\limits_{ab} \int [d\boldsymbol{k}]\partial_{\mu}\partial_{\gamma}\varepsilon_a h^{\alpha}_{ba}h^{\beta}_{cb}f_{ab} d^{\omega_1}_{ab} d^{\omega_{2}}_{ba}
			\end{aligned}
		\end{equation}
		We can extract the resonant part, which contains to the geometry quantities we want
		\begin{equation}
			\begin{aligned}
				\sigma^{\mu\alpha\beta\gamma}_{\text{BCL, m$\times$Q, I}}
				=&-\frac{1}{3!}\frac{2\pi e^4}{2\hbar^4\Omega^{3}}\sum\limits_{\{\alpha, \beta, \gamma\}} \sum\limits_{ab} \int [d\boldsymbol{k}]\partial_{\mu}\partial_{\gamma}\varepsilon_{ab} h^{\alpha}_{ba}h^{\beta}_{ab}f_{ab}\left[d^{\Omega}_{ba}\delta(\Omega + \varepsilon_{ab})\right. \\
				& \left.+ d^{\Omega}_{ab}\delta(2\Omega + \varepsilon_{ab}) + d^{-2\Omega}_{ba}\delta(\Omega + \varepsilon_{ab})\right] \\
				=& -\frac{1}{3!}\frac{\pi e^4}{2\hbar^4\Omega^{3}}\sum\limits_{\{\alpha, \beta, \gamma\}} \sum\limits_{ab} \int [d\boldsymbol{k}]f_{ab}w ^{\mu\gamma}_{ab} \frac{h^{\alpha}_{ba}h^{\beta}_{ab}}{\varepsilon_{ab}}\left[\delta(\Omega + \varepsilon_{ab}) +4 \delta(2\Omega + \varepsilon_{ab})\right] \\
			\end{aligned}
		\end{equation}
        \par
        Sum up both terms, the overall expression is
        \begin{equation}
			\begin{aligned}
				\sigma^{\mu\alpha\beta\gamma}_{\text{BCL, m$\times$Q}}
				=& -\frac{1}{3!}\frac{\pi e^4}{2\hbar^4\Omega^{3}}\sum\limits_{\{\alpha, \beta, \gamma\}} \sum\limits_{ab} \int [d\boldsymbol{k}]f_{ab}w ^{\mu\gamma}_{ab} \frac{h^{\alpha}_{ba}h^{\beta}_{ab}}{\varepsilon_{ab}}\left[5\delta(\Omega + \varepsilon_{ab}) +2 \delta(2\Omega + \varepsilon_{ab})\right] \\
			\end{aligned}
		\end{equation}

		\paragraph{Part 6: (shift vector)$\times$(triple phase product)}
        Both Diagram Set I and Diagram Set II contribute to this term. For Diagram Set I, there are two related sources for such term. (i) Extract the last part of Equation \ref{expansion of second order generalized derivative},
		\begin{equation}
		  \begin{aligned}
				\sigma^{\mu\alpha\beta\gamma}_{\text{BCL, R}\times\text{T}-1} 
                =& \frac{1}{3!}\frac{ie^4}{2 \hbar^4 \omega_1\omega_2\omega_3}\sum\limits_{\{\alpha, \beta, \gamma\}}\sum\limits_{\{(\alpha, \omega_1), (\beta, \omega_2), (\gamma, \omega_3)\}} \sum\limits_{a\neq b\neq c} \int [d\boldsymbol{k}]f_{ab}h^{\alpha}_{ba} \\
				&\left(\frac{h^{\beta}_{ac}h^{\gamma}_{cb}}{\varepsilon_{ac}}R^{\mu, \beta}_{ac}+ \frac{h^{\beta}_{ac}h^{\gamma}_{cb}}{\varepsilon_{ac}}R^{\mu, \gamma}_{cb} - \frac{h^{\gamma}_{ac}h^{\beta}_{cb}}{\varepsilon_{cb}}R^{\mu, \gamma}_{ac}+ \frac{h^{\gamma}_{ac}h^{\beta}_{cb}}{\varepsilon_{cb}}R^{\mu, \beta}_{cb}\right)\left(-i\pi\delta(\varepsilon_{ab} + \omega_1)\right) \\
				=& \frac{1}{3!}\frac{i\pi e^4}{2\hbar^4\Omega^3}\sum\limits_{\{\alpha, \beta, \gamma\}}\sum\limits_{a\neq b\neq c} \int [d\boldsymbol{k}]f_{ab}\left(\frac{1}{\varepsilon_{cb}} - \frac{1}{\varepsilon_{ac}}\right)\\
				&\left[2T^{\alpha\beta\gamma}_{abc}\left(R^{\mu, \gamma}_{ac} + R^{\mu, \beta}_{cb}\right)\delta(\varepsilon_{ab} + \Omega) - \left(T^{\alpha\beta\gamma}_{abc}\right)^* \left(R^{\mu, \beta}_{bc} + R^{\mu, \gamma}_{ca}\right)\delta(\varepsilon_{ab} + 2\Omega)\right]
		  \end{aligned}
		\end{equation}
		\par
		(ii) Extract the second part of Equation \ref{expansion of first order generalized derivative} and combine it with multi-band parts in $h^{\alpha\beta}_{ba}$ expansion.
		\begin{equation}
		  \begin{aligned}
				\sigma^{\mu\alpha\beta\gamma}_{\text{BCL, R}\times\text{T-2}} =& \frac{1}{3!}\frac{ie^4}{2\hbar^4\omega_1\omega_2\omega_3}\sum\limits_{\{\alpha, \beta, \gamma\}}\sum\limits_{\{(\alpha, \omega_1), (\beta, \omega_2), (\gamma, \omega_3)\}} \sum\limits_{a\neq b\neq c} \int [d\boldsymbol{k}]f_{ab}\\
				&\left(\varepsilon_{ca}r^{\alpha}_{bc}r^{\beta}_{ca} - \varepsilon_{bc}r^{\beta}_{bc}r^{\alpha}_{ca}\right)\varepsilon_{ab}R^{\mu, \gamma}_{ab}r^{\gamma}_{ab}\left(-i\pi\delta(\varepsilon_{ab} + \omega_{12}) 	\right) \\
				=& -\frac{1}{3!}\frac{i\pi e^4}{2\hbar^4\Omega^3}\sum\limits_{\{\alpha, \beta, \gamma\}} \sum\limits_{a\neq b\neq c} \int [d\boldsymbol{k}]f_{ba}\left(\frac{1}{\varepsilon_{cb}} - \frac{1}{\varepsilon_{ac}}\right) \\
                &\left[2R^{\mu, \alpha}_{ba}T^{\alpha\beta\gamma}_{abc} \delta(\varepsilon_{ab} + \Omega) +R^{\mu, \alpha}_{ab}\left(T^{\alpha\beta\gamma}_{abc}\right)^* \delta(\varepsilon_{ab} + 2\Omega)  \right]\\
		  \end{aligned}
		\end{equation}
		Sum up both terms, the contribution from Diagram Set I is
		\begin{equation}
            \label{shift current RT, I, 1S}
		  \begin{aligned}
				\sigma^{\mu\alpha\beta\gamma}_{\text{BCL, R}\times\text{T, I, 1S}}
				=& \frac{1}{3!}\frac{i\pi e^4}{2\hbar^4\Omega^3}\sum\limits_{\{\alpha, \beta, \gamma\}}\sum\limits_{a\neq b\neq c} \int [d\boldsymbol{k}]f_{ab}\left(\frac{1}{\varepsilon_{cb}} - \frac{1}{\varepsilon_{ac}}\right)\\
				&\left[2T^{\alpha\beta\gamma}_{abc}\left(R^{\mu, \gamma}_{ac} + R^{\mu, \beta}_{cb} - R^{\mu, \alpha}_{ba}\right)\delta(\varepsilon_{ab} + \Omega) \right.\\
                &\left. - \left(T^{\alpha\beta\gamma}_{abc}\right)^* \left(R^{\mu, \beta}_{bc} + R^{\mu, \gamma}_{ca} - R^{\mu, \alpha}_{ab}\right)\delta(\varepsilon_{ab} + 2\Omega)\right]
		  \end{aligned}
		\end{equation}
        It's obvious that overall contribution from Diagram Set I all has one singularity
        \par
        For Diagram Set II, we should be more careful since there exist both part with one singularity and part with double singularities. We start by deriving the overall expression for the geometry quantities we want
        \begin{equation}
		  \begin{aligned}
				\sigma^{\mu\alpha\beta\gamma}_{\text{BCL, R}\times\text{T, II}}
				=&\frac{1}{3!}\frac{ie^4}{\hbar^4\omega_1\omega_2\omega_3}\sum\limits_{\{\alpha, \beta, \gamma\}}\sum\limits_{\{(\alpha, \omega_1), (\beta, \omega_2), (\gamma, \omega_3)\}} \sum\limits_{abc} \int [d\boldsymbol{k}] \\
				&\left(-iR^{\mu, \gamma}_{ac}\frac{h^{\gamma}_{ac}}{\varepsilon_{ac}}\right)h^{\alpha}_{ba}h^{\beta}_{cb}\left[f_a d^{\omega_1}_{ab} d^{\omega_{12}}_{ac} - f_b d^{\omega_1}_{ab}d^{\omega_{2}}_{bc} + f_c d^{\omega_{12}}_{ac}d^{\omega_2}_{bc}\right] \\
                =&-\frac{1}{3!}\frac{e^4}{\hbar^4\Omega^3} \sum\limits_{\{\alpha, \beta, \gamma\}} \sum\limits_{a\neq b \neq c} \int [d\boldsymbol{k}] f_{ab}\left\{T^{\alpha\beta\gamma}_{abc} d^{\Omega}_{ab} \left[R^{\mu, \gamma}_{ac}\left(d^{2\Omega}_{ac} + d^{-\Omega}_{ac}\right) -R^{\mu, \beta}_{cb}\left(d^{2\Omega}_{cb} + d^{-\Omega}_{cb}\right) \right] \right. \\
                &\left.+ \left(T^{\alpha\beta\gamma}_{abc}\right)^* d^{-2\Omega}_{ba} \left[R^{\mu, \gamma}_{ca}d^{-\Omega}_{ca} -R^{\mu, \beta}_{bc}d^{-\Omega}_{bc} \right]\right\}
	   	\end{aligned}
		\end{equation}	
        We can further divide this overall expression according to the number of Dirac delta function within. The part containing one singularity is
        \begin{equation}
            \label{shift current RT, II, 1S}
		  \begin{aligned}
				&\sigma^{\mu\alpha\beta\gamma}_{\text{BCL, R}\times\text{T, II, 1S}} \\
                =&\frac{1}{3!}\frac{i\pi e^4}{\hbar^4\Omega^3} \sum\limits_{\{\alpha, \beta, \gamma\}} \sum\limits_{a\neq b \neq c} \int [d\boldsymbol{k}] f_{ab} \\
                &\left\{T^{\alpha\beta\gamma}_{abc} \left\{\mathcal{P.V.} \frac{1}{\varepsilon_{ab} + \Omega}\left[R^{\mu, \gamma}_{ac}\left(\delta(\varepsilon_{ac} + 2\Omega) + \delta(\varepsilon_{ac} - \Omega)\right) -R^{\mu, \beta}_{cb}\left(\delta(\varepsilon_{cb} + 2\Omega) + \delta(\varepsilon_{cb} - \Omega)\right) \right] \right.\right.\\
                &\left.\left.+\delta(\varepsilon_{ab} + \Omega)\left[R^{\mu, \gamma}_{ac}\left(\mathcal{P.V.} \frac{1}{\varepsilon_{ac} + 2\Omega} + \mathcal{P.V.} \frac{1}{\varepsilon_{ac} - \Omega}\right)-R^{\mu, \beta}_{cb}\left(\mathcal{P.V.} \frac{1}{\varepsilon_{cb} + 2\Omega} + \mathcal{P.V.} \frac{1}{\varepsilon_{cb} - \Omega}\right) \right]\right\} \right. \\
                &\left.+ \left(T^{\alpha\beta\gamma}_{abc}\right)^* \left\{\mathcal{P.V.} \frac{1}{\varepsilon_{ba} - 2\Omega} \left[R^{\mu, \gamma}_{ca}\delta(\varepsilon_{ca} - \Omega) -R^{\mu, \beta}_{bc}\delta(\varepsilon_{bc} - \Omega) \right]\right.\right. \\
                &\left.\left.+ \delta(\varepsilon_{ab} + 2\Omega) \left[R^{\mu, \gamma}_{ca}\mathcal{P.V.} \frac{1}{\varepsilon_{ca} - \Omega} -R^{\mu, \beta}_{bc}\frac{1}{\varepsilon_{bc} - \Omega} \right]\right\}\right\} \\
                =&\frac{1}{3!}\frac{i\pi e^4}{\hbar^4\Omega^3} \sum\limits_{\{\alpha, \beta, \gamma\}} \sum\limits_{a\neq b \neq c} \int [d\boldsymbol{k}] f_{ab} \\
                &\left[ T^{\alpha\beta\gamma}_{abc} \left(R^{\mu, \gamma}_{ac} + R^{\mu, \beta}_{cb} - R^{\mu, \alpha}_{ba}\right)\left(\mathcal{P.V.} \frac{1}{\varepsilon_{ac} + 2\Omega} + \mathcal{P.V.} \frac{1}{\varepsilon_{ac} - \Omega} \right)\delta(\varepsilon_{ab} + \Omega) \right.\\
                &\left.- \left(T^{\alpha\beta\gamma}_{abc}\right)^* \left(R^{\mu, \beta}_{bc} + R^{\mu, \gamma}_{ca} - R^{\mu, \alpha}_{ab}\right)\mathcal{P.V.} \frac{1}{\varepsilon_{ac} + \Omega}\delta(\varepsilon_{ab} + 2\Omega)\right]
	   	\end{aligned}
		\end{equation}
        The part containing double singularities is
        \begin{equation}
            \label{shift current RT, II, 2S}
		  \begin{aligned}
				\sigma^{\mu\alpha\beta\gamma}_{\text{BCL, R}\times\text{T, II, 2S}}
                =&\frac{1}{3!}\frac{\pi^2 e^4}{\hbar^4\Omega^3} \sum\limits_{\{\alpha, \beta, \gamma\}} \sum\limits_{a\neq b \neq c} \int [d\boldsymbol{k}] f_{ab} \\
                &\left\{T^{\alpha\beta\gamma}_{abc} \delta(\varepsilon_{ab} + \Omega)\left[R^{\mu, \gamma}_{ac}\left(\delta(\varepsilon_{ac} + 2\Omega) + \delta(\varepsilon_{ac} - \Omega)\right) -R^{\mu, \beta}_{cb}\left(\delta(\varepsilon_{cb} + 2\Omega) + \delta(\varepsilon_{cb} - \Omega)\right) \right] \right. \\
                &\left.+ \left(T^{\alpha\beta\gamma}_{abc}\right)^* \delta(\varepsilon_{ab} + 2\Omega) \left[R^{\mu, \gamma}_{ca}\delta(\varepsilon_{ca} - \Omega) -R^{\mu, \beta}_{bc}\delta(\varepsilon_{bc} - \Omega) \right]\right\} \\
                =&\frac{1}{3!}\frac{\pi^2 e^4}{\hbar^4\Omega^3} \sum\limits_{\{\alpha, \beta, \gamma\}} \sum\limits_{a\neq b \neq c} \int [d\boldsymbol{k}] T^{\alpha\beta\gamma}_{abc}\\
                &\left[f_{ab}\left(R^{\mu, \gamma}_{ac} - R^{\mu, \beta}_{cb}\right)+f_{bc}\left(R^{\mu, \alpha}_{ba} - R^{\mu, \gamma}_{ac}\right)+f_{ca}\left(R^{\mu, \beta}_{cb} - R^{\mu, \alpha}_{ba}\right)\right]\delta(\varepsilon_{ab} + \Omega)\delta(\varepsilon_{bc} + \Omega)
	   	\end{aligned}
        \end{equation}
        \par
        The overall expression for terms with one singularity can be obtained by adding up Equation \ref{shift current RT, I, 1S} and \ref{shift current RT, II, 1S}.
        \begin{equation}
		  \begin{aligned}
				&\sigma^{\mu\alpha\beta\gamma}_{\text{BCL, R}\times\text{T, 1S}} \\
                =& \frac{1}{3!}\frac{i\pi e^4}{\hbar^4\Omega^3}\sum\limits_{\{\alpha, \beta, \gamma\}}\sum\limits_{a\neq b\neq c} \int [d\boldsymbol{k}] \frac{1}{2}f_{ab}\left(\frac{1}{\varepsilon_{cb}} - \frac{1}{\varepsilon_{ac}}\right)\left[2T^{\alpha\beta\gamma}_{abc}\left(R^{\mu, \gamma}_{ac} + R^{\mu, \beta}_{cb} - R^{\mu, \alpha}_{ba}\right)\delta(\varepsilon_{ab} + \Omega) \right.\\
                &\left. - \left(T^{\alpha\beta\gamma}_{abc}\right)^* \left(R^{\mu, \beta}_{bc} + R^{\mu, \gamma}_{ca} - R^{\mu, \alpha}_{ab}\right)\delta(\varepsilon_{ab} + 2\Omega)\right] \\
                &+ f_{ab}\left[ T^{\alpha\beta\gamma}_{abc} \left(R^{\mu, \gamma}_{ac} + R^{\mu, \beta}_{cb} - R^{\mu, \alpha}_{ba}\right)\left(\mathcal{P.V.} \frac{1}{\varepsilon_{ac} + 2\Omega} + \mathcal{P.V.} \frac{1}{\varepsilon_{ac} - \Omega} \right)\delta(\varepsilon_{ab} + \Omega) \right.\\
                &\left.- \left(T^{\alpha\beta\gamma}_{abc}\right)^* \left(R^{\mu, \beta}_{bc} + R^{\mu, \gamma}_{ca} - R^{\mu, \alpha}_{ab}\right)\mathcal{P.V.} \frac{1}{\varepsilon_{ac} + \Omega}\delta(\varepsilon_{ab} + 2\Omega)\right]
	   	\end{aligned}
		\end{equation}        
        The overall expression for terms with double singularity is exactly Equation \ref{shift current RT, II, 2S}.
        \begin{equation}
		  \begin{aligned}
				\sigma^{\mu\alpha\beta\gamma}_{\text{BCL, R}\times\text{T, 2S}}
                =&\frac{1}{3!}\frac{\pi^2 e^4}{\hbar^4\Omega^3} \sum\limits_{\{\alpha, \beta, \gamma\}} \sum\limits_{a\neq b \neq c} \int [d\boldsymbol{k}] T^{\alpha\beta\gamma}_{abc}\\
                &\left[f_{ab}\left(R^{\mu, \gamma}_{ac} - R^{\mu, \beta}_{cb}\right)+f_{bc}\left(R^{\mu, \alpha}_{ba} - R^{\mu, \gamma}_{ac}\right)+f_{ca}\left(R^{\mu, \beta}_{cb} - R^{\mu, \alpha}_{ba}\right)\right]\delta(\varepsilon_{ab} + \Omega)\delta(\varepsilon_{bc} + \Omega)
	   	\end{aligned}
        \end{equation}


		\paragraph{Part 7: (group velocity)$\times$(triple phase product)} Both Diagram Set I and Diagram Set II contribute to this term. For Diagram Set I, there are two sources for such term. (i) extract the fifth part of Equation \ref{expansion of second order generalized derivative}.
		\begin{equation}
			\begin{aligned}
				\sigma^{\mu\alpha\beta\gamma}_{\text{BCL, }\Delta\times\text{T-1}} =& \frac{1}{3!}\frac{ie^4}{2\hbar^4\omega_1\omega_2\omega_3}\sum\limits_{\{\alpha, \beta, \gamma\}}\sum\limits_{\{(\alpha, \omega_1), (\beta, \omega_2), (\gamma, \omega_3)\}} \sum\limits_{a\neq b\neq c} \int [d\boldsymbol{k}]f_{ab}h^{\alpha}_{ba} \\
                &\left(-\Delta^{\mu}_{cb}\frac{h^{\beta}_{ac}h^{\gamma}_{cb}}{\varepsilon_{ac}\varepsilon_{cb}} + \Delta^{\mu}_{ac}\frac{h^{\gamma}_{ac}h^{\beta}_{cb}}{\varepsilon_{ac}\varepsilon_{cb}}\right)d^{\omega_1}_{ab} \\
				=&\frac{1}{3!}\frac{\pi e^4}{2\hbar^4\Omega^3}\sum\limits_{\{\alpha, \beta, \gamma\}}\sum\limits_{a\neq b\neq c} \int [d\boldsymbol{k}] f_{ab}\frac{\Delta^{\mu}_{cb} - \Delta^{\mu}_{ac}}{\varepsilon_{ac}\varepsilon_{cb}}\left[2T^{\alpha\beta\gamma}_{abc} \delta(\varepsilon_{ab} + \Omega) - \left(T^{\alpha\beta\gamma}_{abc}\right)^* \delta(\varepsilon_{ab} + 2\Omega)\right] \\
			\end{aligned}
		\end{equation}
		(ii) Extract the first part of Equation \ref{expansion of first order generalized derivative} and combine it with multi-band parts in $h^{\alpha\beta}_{ba}$ expansion.
		\begin{equation}
			\begin{aligned}
				\sigma^{\mu\alpha\beta\gamma}_{\text{BCL, }\Delta\times\text{T-2}} =& \frac{1}{3!}\frac{ie^4}{2\hbar^4\omega_1\omega_2\omega_3}\sum\limits_{\{\alpha, \beta, \gamma\}}\sum\limits_{\{(\alpha, \omega_1), (\beta, \omega_2), (\gamma, \omega_3)\}} \sum\limits_{a\neq b\neq c} \int [d\boldsymbol{k}]f_{ab}\Delta^{\mu}_{ab}\frac{h^{\gamma}_{ab}}{\varepsilon_{ab}}\left(-\frac{h^{\alpha}_{bc}h^{\beta}_{ca}}{\varepsilon_{bc}} + \frac{h^{\beta}_{bc}h^{\alpha}_{ca}}{\varepsilon_{ca}}\right)d^{\omega_{12}}_{ab} \\
				=&\frac{1}{3!}\frac{\pi e^4}{2\hbar^4\Omega^3}\sum\limits_{\{\alpha, \beta, \gamma\}}\sum\limits_{a\neq b\neq c} \int [d\boldsymbol{k}] f_{ab}\Delta^{\mu}_{ab}\left(\frac{1}{\varepsilon_{ac}\varepsilon_{ba}} - \frac{1}{\varepsilon_{cb}\varepsilon_{ba}}\right) \\
                &\left[2T^{\alpha\beta\gamma}_{abc} \delta(\varepsilon_{ab} + \Omega) - \left(T^{\alpha\beta\gamma}_{abc}\right)^* \delta(\varepsilon_{ab} + 2\Omega)\right] \\
			\end{aligned}
		\end{equation}
		Sum up both terms, we can obtain the contribution from Diagram Set I
		\begin{equation}
            \label{shift current DeltaT, I, 1S}
		  \begin{aligned}
				\sigma^{\mu\alpha\beta\gamma}_{\text{BCL, }\Delta\times\text{T, I, 1S}}
				=&-\frac{1}{3!}\frac{\pi e^4}{2\hbar^4\Omega^3}\sum\limits_{\{\alpha, \beta, \gamma\}}\sum\limits_{a\neq b\neq c} \int [d\boldsymbol{k}] f_{ab}\left(\frac{1}{\varepsilon_{cb}} - \frac{1}{\varepsilon_{ac}}\right)\left(\frac{\Delta^{\mu}_{cb} + \Delta^{\mu}_{ac}}{\varepsilon_{cb} - \varepsilon_{ac}} - \frac{\Delta^{\mu}_{ba}}{\varepsilon_{ba}}\right) \\
                &\left[2T^{\alpha\beta\gamma}_{abc} \delta(\varepsilon_{ab} + \Omega) - \left(T^{\alpha\beta\gamma}_{abc}\right)^* \delta(\varepsilon_{ab} + 2\Omega)\right] \\
		  \end{aligned}
		\end{equation}
        The contribution from Diagram Set I only contains one singularity.
        \par
        For Diagram Set II, there also exist both part with one singularity and part with double singularities. The overall expression for this term can be written as
        \begin{equation}
			\begin{aligned}
				\sigma^{\mu\alpha\beta\gamma}_{\text{BCL,  $\Delta\times$T, II}}
				=&-\frac{1}{3!}\frac{ie^4}{\hbar^4\Omega^3}\sum\limits_{\{\alpha, \beta, \gamma\}}\sum\limits_{a \neq b \neq c} \int [d\boldsymbol{k}]  f_{ab}\left\{T^{\alpha\beta\gamma}_{abc}d^{\Omega}_{ab}\left[\frac{\Delta^{\mu}_{ac}}{\varepsilon_{ac}}\left(d^{2\Omega}_{ac} + d^{-\Omega}_{ac}\right) - \frac{\Delta^{\mu}_{cb}}{\varepsilon_{cb}}\left(d^{2\Omega}_{cb} + d^{-\Omega}_{cb}\right)\right]\right. \\
				&\left. - \left(T^{\alpha\beta\gamma}_{abc}\right)^* d^{-2\Omega}_{ba}\left(\frac{\Delta^{\mu}_{bc}}{\varepsilon_{bc}}d^{-\Omega}_{bc} - \frac{\Delta^{\mu}_{ca}}{\varepsilon_{ca}}d^{-\Omega}_{ca}\right)\right\}\\
			\end{aligned}
		\end{equation}
        The part with one singularity corresponds to part with one Dirac delta function
        \begin{equation}
            \label{shift current DeltaT, II, 1S}
		  \begin{aligned}
				&\sigma^{\mu\alpha\beta\gamma}_{\text{BCL,  $\Delta\times$T, II, 1S}} \\
                =&-\frac{1}{3!}\frac{\pi e^4}{\hbar^4\Omega^3} \sum\limits_{\{\alpha, \beta, \gamma\}} \sum\limits_{a\neq b \neq c} \int [d\boldsymbol{k}] f_{ab} \\
                &\left\{T^{\alpha\beta\gamma}_{abc} \left\{\mathcal{P.V.} \frac{1}{\varepsilon_{ab} + \Omega}\left[\frac{\Delta^{\mu}_{ac}}{\varepsilon_{ac}}\left(\delta(\varepsilon_{ac} + 2\Omega) + \delta(\varepsilon_{ac} - \Omega)\right) -\frac{\Delta^{\mu}_{cb}}{\varepsilon_{cb}}\left(\delta(\varepsilon_{cb} + 2\Omega) + \delta(\varepsilon_{cb} - \Omega)\right) \right] \right.\right.\\
                &\left.\left.+\delta(\varepsilon_{ab} + \Omega)\left[\frac{\Delta^{\mu}_{ac}}{\varepsilon_{ac}}\left(\mathcal{P.V.} \frac{1}{\varepsilon_{ac} + 2\Omega} + \mathcal{P.V.} \frac{1}{\varepsilon_{ac} - \Omega}\right)-\frac{\Delta^{\mu}_{cb}}{\varepsilon_{cb}}\left(\mathcal{P.V.} \frac{1}{\varepsilon_{cb} + 2\Omega} + \mathcal{P.V.} \frac{1}{\varepsilon_{cb} - \Omega}\right) \right]\right\} \right. \\
                &\left.+ \left(T^{\alpha\beta\gamma}_{abc}\right)^* \left\{\mathcal{P.V.} \frac{1}{\varepsilon_{ba} - 2\Omega} \left[\frac{\Delta^{\mu}_{ac}}{\varepsilon_{ac}}\delta(\varepsilon_{ca} - \Omega) \frac{\Delta^{\mu}_{cb}}{\varepsilon_{cb}}\delta(\varepsilon_{bc} - \Omega) \right]\right.\right. \\
                &\left.\left.+ \delta(\varepsilon_{ab} + 2\Omega) \left[\frac{\Delta^{\mu}_{ac}}{\varepsilon_{ac}}\mathcal{P.V.} \frac{1}{\varepsilon_{ca} - \Omega} -\frac{\Delta^{\mu}_{cb}}{\varepsilon_{cb}}\frac{1}{\varepsilon_{bc} - \Omega} \right]\right\}\right\} \\
                =&-\frac{1}{3!}\frac{\pi e^4}{\hbar^4\Omega^3}  \sum\limits_{\{\alpha, \beta, \gamma\}} \sum\limits_{a\neq b \neq c} \int [d\boldsymbol{k}] f_{ab} \left(\frac{\Delta^{\mu}_{ac}}{\varepsilon_{ac}} + \frac{\Delta^{\mu}_{cb}}{\varepsilon_{cb}} - \frac{\Delta^{\mu}_{ba}}{\varepsilon_{ba}}\right)\\
                &\left[ T^{\alpha\beta\gamma}_{abc} \left(\mathcal{P.V.} \frac{1}{\varepsilon_{ac} + 2\Omega} + \mathcal{P.V.} \frac{1}{\varepsilon_{ac} - \Omega} \right)\delta(\varepsilon_{ab} + \Omega) - \left(T^{\alpha\beta\gamma}_{abc}\right)^* \mathcal{P.V.} \frac{1}{\varepsilon_{ac} + \Omega}\delta(\varepsilon_{ab} + 2\Omega)\right]
	   	\end{aligned}
		\end{equation}        
        The part with double singularities is
        \begin{equation}
            \label{shift current DeltaT, II, 2S}
		  \begin{aligned}
				\sigma^{\mu\alpha\beta\gamma}_{\text{BCL,  $\Delta\times$T, II, 2S}} 
                =&\frac{1}{3!}\frac{i\pi^2 e^4}{\hbar^4\Omega^3} \sum\limits_{\{\alpha, \beta, \gamma\}} \sum\limits_{a\neq b \neq c} \int [d\boldsymbol{k}] f_{ab} \\
                &\left\{T^{\alpha\beta\gamma}_{abc} \delta(\varepsilon_{ab} + \Omega)\left[\frac{\Delta^{\mu}_{ac}}{\varepsilon_{ac}}\left(\delta(\varepsilon_{ac} + 2\Omega) + \delta(\varepsilon_{ac} - \Omega)\right) - \frac{\Delta^{\mu}_{cb}}{\varepsilon_{cb}}\left(\delta(\varepsilon_{cb} + 2\Omega) + \delta(\varepsilon_{cb} - \Omega)\right) \right] \right. \\
                &\left.+ \left(T^{\alpha\beta\gamma}_{abc}\right)^* \delta(\varepsilon_{ab} + 2\Omega) \left[\frac{\Delta^{\mu}_{ac}}{\varepsilon_{ac}}\delta(\varepsilon_{ca} - \Omega) - \frac{\Delta^{\mu}_{cb}}{\varepsilon_{cb}}\delta(\varepsilon_{bc} - \Omega) \right]\right\} \\
                =&\frac{1}{3!}\frac{\pi^2 e^4}{\hbar^4\Omega^3} \sum\limits_{\{\alpha, \beta, \gamma\}} \sum\limits_{a\neq b \neq c} \int [d\boldsymbol{k}] T^{\alpha\beta\gamma}_{abc}\\
                &\left[f_{ab}\left(\frac{\Delta^{\mu}_{ac}}{\varepsilon_{ac}} -  \frac{\Delta^{\mu}_{cb}}{\varepsilon_{cb}}\right)+f_{bc}\left(\frac{\Delta^{\mu}_{ba}}{\varepsilon_{ba}} - \frac{\Delta^{\mu}_{ac}}{\varepsilon_{ac}}\right)+f_{ca}\left( \frac{\Delta^{\mu}_{cb}}{\varepsilon_{cb}} - \frac{\Delta^{\mu}_{ba}}{\varepsilon_{ba}}\right)\right]\delta(\varepsilon_{ab} + \Omega)\delta(\varepsilon_{bc} + \Omega)
	   	\end{aligned}
        \end{equation}
        \par
        The overall expression for terms with one singularity can be obtained by adding up Equation \ref{shift current DeltaT, I, 1S} and \ref{shift current DeltaT, II, 1S}.
        The part with one singularity corresponds to part with one Dirac delta function
        \begin{equation}
		  \begin{aligned}
				&\sigma^{\mu\alpha\beta\gamma}_{\text{BCL,  $\Delta\times$T, 1S}} \\
                =&-\frac{1}{3!}\frac{\pi e^4}{\hbar^4\Omega^3}\sum\limits_{\{\alpha, \beta, \gamma\}}\sum\limits_{a\neq b\neq c} \int [d\boldsymbol{k}] \frac{1}{2}f_{ab}\left(\frac{1}{\varepsilon_{cb}} - \frac{1}{\varepsilon_{ac}}\right)\left(\frac{\Delta^{\mu}_{cb} + \Delta^{\mu}_{ac}}{\varepsilon_{cb} - \varepsilon_{ac}} - \frac{\Delta^{\mu}_{ba}}{\varepsilon_{ba}}\right) \\
                &\left[2T^{\alpha\beta\gamma}_{abc} \delta(\varepsilon_{ab} + \Omega) - \left(T^{\alpha\beta\gamma}_{abc}\right)^* \delta(\varepsilon_{ab} + 2\Omega)\right] \\
                &+ f_{ab} \left(\frac{\Delta^{\mu}_{ac}}{\varepsilon_{ac}} + \frac{\Delta^{\mu}_{cb}}{\varepsilon_{cb}} - \frac{\Delta^{\mu}_{ba}}{\varepsilon_{ba}}\right)\\
                &\left[ T^{\alpha\beta\gamma}_{abc} \left(\mathcal{P.V.} \frac{1}{\varepsilon_{ac} + 2\Omega} + \mathcal{P.V.} \frac{1}{\varepsilon_{ac} - \Omega} \right)\delta(\varepsilon_{ab} + \Omega) - \left(T^{\alpha\beta\gamma}_{abc}\right)^* \mathcal{P.V.} \frac{1}{\varepsilon_{ac} + \Omega}\delta(\varepsilon_{ab} + 2\Omega)\right]
	   	\end{aligned}
		\end{equation}              
        The overall expression for terms with double singularities is exactly Equation \ref{shift current DeltaT, II, 2S}.
        \begin{equation}
		  \begin{aligned}
				\sigma^{\mu\alpha\beta\gamma}_{\text{BCL,  $\Delta\times$T, 2S}} 
                =&\frac{1}{3!}\frac{\pi^2 e^4}{\hbar^4\Omega^3} \sum\limits_{\{\alpha, \beta, \gamma\}} \sum\limits_{a\neq b \neq c} \int [d\boldsymbol{k}] T^{\alpha\beta\gamma}_{abc}\\
                &\left[f_{ab}\left(\frac{\Delta^{\mu}_{ac}}{\varepsilon_{ac}} -  \frac{\Delta^{\mu}_{cb}}{\varepsilon_{cb}}\right)+f_{bc}\left(\frac{\Delta^{\mu}_{ba}}{\varepsilon_{ba}} - \frac{\Delta^{\mu}_{ac}}{\varepsilon_{ac}}\right)+f_{ca}\left( \frac{\Delta^{\mu}_{cb}}{\varepsilon_{cb}} - \frac{\Delta^{\mu}_{ba}}{\varepsilon_{ba}}\right)\right]\delta(\varepsilon_{ab} + \Omega)\delta(\varepsilon_{bc} + \Omega)
	   	\end{aligned}
        \end{equation}
_old
